# Supplementary material for: Enabling Safety for Aerial Robots: Planning and Control Architectures
Source: arXiv:2504.08601 source file (2025-04-11)
Supplement: Supplementary file 1 [file Appendix.tex]

% \textcolor{red}{Please Skip for now}

% \subsection{Figures}

% \subsubsection{Figure 1}

% Figure 1 serves as the introductory paper. This figure should help readers understand the terms spatial variability, temporal variability and how some parts of the environment has faster temporal variability and some other regions have slower temporal variability.  Should I be more general in my explanation. I can probably talk wind as the quantity of interest and design an environment with these features:
% \begin{itemize}
%     \item Over water, the wind speed is much higher than the land. So, the spatial variability makes sense
%     \item I have am idea about how I want to show the environment. If I want to show the temporal variation maybe I can show that using the 1D plots I have in the notebook
    
% \end{itemize}
